# Supplementary material for: Learning to Detect Mobile Objects from LiDAR Scans Without Labels
Source: arXiv:2203.15882 source file (2022-03-29)
Supplement: Supplementary file 1 [file self_training_progression.tex]

{
\begin{figure*}[ht]
   \centering
\begin{tabular}{ccc|c}
% \ourmethod (R0) & \ourmethod (R5) & \ourmethod (R10) & \ourmethod (R19) & Ground Truth  \\
\ourmethod (R0) & \ourmethod (R5) & \ourmethod (R10) & Ground Truth  \\
% \hline\hline

\includegraphics[width=0.24\textwidth]{supp_figures/000699_p0_lidar.png}&
\includegraphics[width=0.24\textwidth]{supp_figures/000699_p1_lidar.png}&
\includegraphics[width=0.24\textwidth]{supp_figures/000699_p2_lidar.png}&
\includegraphics[width=0.24\textwidth]{supp_figures/000699_gt_lidar.png} \\

\includegraphics[width=0.24\textwidth]{supp_figures/012914_p0_lidar.png}&
\includegraphics[width=0.24\textwidth]{supp_figures/012914_p1_lidar.png}&
\includegraphics[width=0.24\textwidth]{supp_figures/012914_p2_lidar.png}&
\includegraphics[width=0.24\textwidth]{supp_figures/012914_gt_lidar.png} 

\end{tabular}

\caption{Visual comparison of self-training iteration results on \ourmethod.
% For Satellite$\rightarrow$Map (top 3) our method out-performs the baselines visually and is very close to the ground truth. Map$\rightarrow$Satellite (bottom 3) our method reduces the ghosting artifacts present in the other methods.
}
\label{fig:st_progression}
\vspace{-15pt}
\end{figure*}
}
